# Supplementary material for: Optimized Quantification of Spin Relaxation Times in the Hybrid State
Source: arXiv:1703.00481 ancillary file (2018-12-03)
Supplement: Supplementary file 1 [file bHSFP_OCT_Supplements.pdf]

SUPPLEMENTARY MATERIAL

# Optimization of Hybrid-State Free Precession Sequences for quantifying MR Relaxation Times


Jakob Assländer*[1,2] | Riccardo Lattanzi[1,2,3] | Daniel K. Sodickson[1,2,3] | Martijn A. Cloos[1,2]

[1]Center for Biomedical Imaging, Dept. of Radiology, New York University School of Medicine, NY, USA
[2]Center for Advanced Imaging Innovation and Research (CAI2R), Dept. of Radiology, New York University School of Medicine, NY, USA
[3]The Sackler Institute of Graduate Biomedical Sciences, New York University School of Medicine, NY, USA


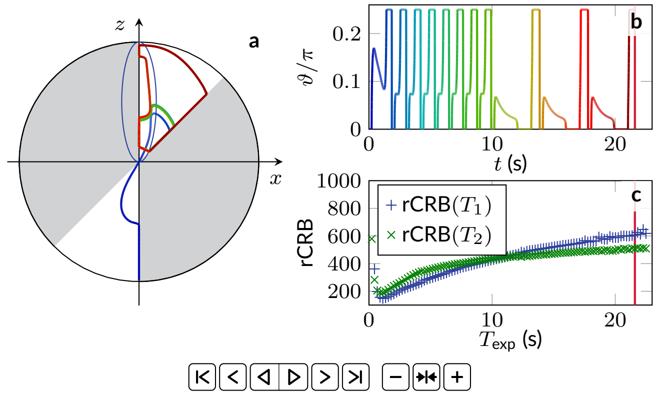


**Supporting Figure S1** The influence of the duration the experiment $T_{\text{exp}}$ on the spin ensemble trajectory is analyzed at the example of the joint optimization for $T_1$ and $T_2$. Note that essentially $T_{\text{exp}}/T_2$ is varied by keeping $T_2 = 65$ ms fixed. *In order to run the animation, please use a PDF-viewer capable of Java-Script, such as the Adobe Acrobat Reader.*

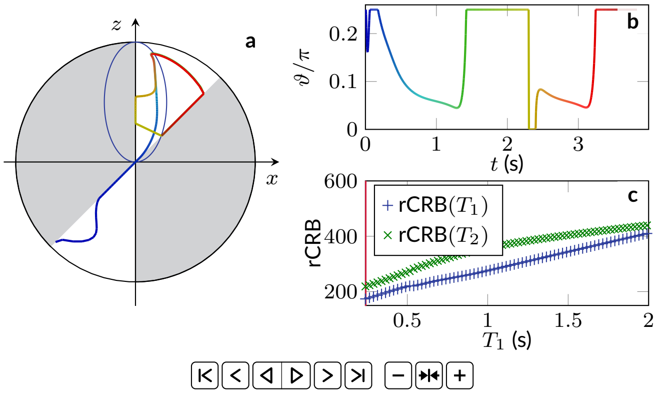


**Supporting Figure S2** The influence of $T_1$ on the spin ensemble trajectory is analyzed at the example of the joint optimization for $T_1$ and $T_2$. Note that essentially $T_1/T_2$ is varied by keeping $T_2 = 65$ ms fixed. *In order to run the animation, please use a PDF-viewer capable of Java-Script, such as the Adobe Acrobat Reader.*

## S1 | SPIN DYNAMICS ON THE BLOCH SPHERE

To highlight the dependencies of the Bloch equations in hybrid state, Eq. (1) can be multiplied by $T_1$. Substituting $t \to \tau = t/T_2$, defining $\dot{r}(\tau) = dr(\tau)/d\tau$, and applying the chain rule results in

$$\frac{T_1}{T_2}\dot{r}(\tau) = \cos\vartheta(\tau) - r(\tau)\left(\cos^2\vartheta(\tau) + \frac{T_1}{T_2}\sin^2\vartheta(\tau)\right), \qquad \text{(S1)}$$

which demonstrates that the spin dynamics depends only on the dimensionless ratios $T_1/T_2$ and $t/T_2$. This allows one to generalize the $\vartheta$-patterns that result from optimizations with one set of parameters to different sets of parameters that have the same ratio $T_1/T_2$ by adjusting $T_{\text{exp}}$ accordingly. Consequently, a full set of optimized $\vartheta$-patterns are given, e.g., by fixing $T_2$ and optimizing for all required combinations of $T_1$ and $T_{\text{exp}}$. Optimizations along the two axes of this parameter space are depicted in Fig. S1, where $T_1 = 781$ ms and $T_2 = 65$ ms are fixed and $T_{\text{exp}}$ is varied, and in Fig. S2, where $T_{\text{exp}} = 3.8$ s and $T_2 = 65$ ms are fixed and $T_1$ is varied.

## S2 | CORRELATION COEFFICIENTS

In order to relate the Cramér-Rao bound analysis in Fig. 4 to the matching procedures commonly used in MRF, we calculated the correlation coefficient $\beta$ between the dictionary atoms. Fig. S3 depicts the correlation between the fingerprint corresponding $T_1 = 781$ms and $T_2 = 65$ms (red square) and the other fingerprints in the dictionary. These results are in good agreement with the $rCRB$ plots shown in Fig. 4. Optimizing for a single relaxation time results in a comparably narrow peak of high correlation coefficients in the optimized dimension and a broad peak along the other dimension. The broadest peak is observed along $T_2$ in the $T_1$-optimized sequence, which is in agreement with the Cramér-Rao bound analysis (Fig. 4) and the in vivo experiments (Fig. 5). The joint optimization results in narrow peaks along both dimensions and confirms that adding a second relaxation time to the optimization has a very small penalty on the original relaxation time.

Fig. S4 shows maximum intensity projections of the full correlation matrix among all fingerprints in the dictionary. These projections can be understood as the worst case correlations for a single parameter under consideration of all values of the other parameter. The generally larger $rCRB(T_2)$ compared to $rCRB(T_1)$ is reflected by the correlation coefficients, which are scaled equally. The findings confirm that the joint optimization has a performance in encoding $T_1$ and $T_2$ that is comparable to respective specialized sequences. Further, the least precise encoding is along $T_2$ when using the $T_1$-optimized sequence, as already found in the Cramér-Rao bound analysis.

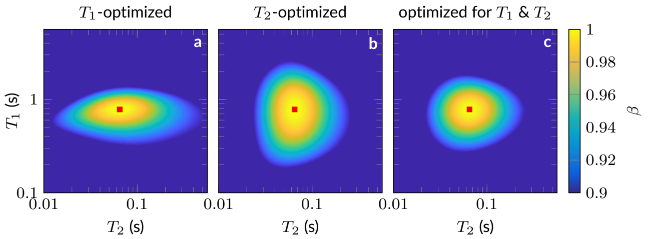


**Supporting Figure S3** The performance of IR-bHSFP optimized with $0 \leq \vartheta \leq \pi/4$ (Fig. 2j-r) is illustrated through plots of the correlation of the fingerprint using the optimization parameters $T_1 = 781$ ms and $T_2 = 65$ ms (red square) with the rest of the parameter space.

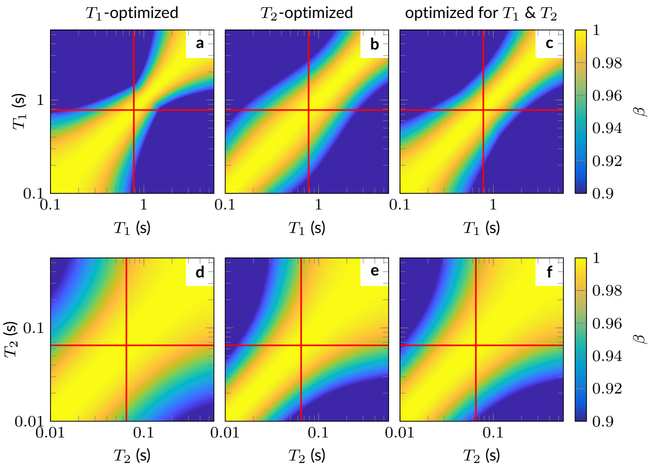


**Supporting Figure S4** The performance of IR-bHSFP optimized with $0 \leq \vartheta \leq \pi/4$ (Fig. 2j-r) is depicted through plots of the correlation coefficient. The correlation matrix was calculated for the entire parameter space. Thereafter, a maximum intensity projection was performed along the $T_2$- (**a**-**d**) and the $T_1$-dimension (**e**-**h**), respectively. The result can be understood as the worst case correlations for a single parameter under consideration of all values of the other parameter. The red lines indicates the set of parameters used for optimizing the patterns.
